# Supplementary material for: A study of Neural networks point source extraction on simulated Fermi/LAT Telescope images
Source: arXiv:2007.04295 source file (2020-07-08)
Supplement: Supplementary file 1 [file app.tex]

\section{Appendix}
\label{sec:app}

%\subsection{Hyper parameter optimisation}

%One of the hyper parameters of our problem is 

\subsection{UNet}
Optimal parameters for the UNet model were selected from the range shown in Table \ref{table:unet_params}. Also, this table shows the resulted metrics for each configuration.

The graph of the loss on the validation set as a result of learning different UNet configurations can be seen in Figure \ref{fig:val_loss}. The largest model shows the lowest loss value throughout the learning process. After the end of the training process, the optimal threshold for each model was selected separately, with which they show the best result on the validation set. Resulted metrics shown in the Table 4 were calculated on the test set.

\begin{figure}[h!]
    \centering
    \includegraphics[scale=0.37]{images/val_loss.png}
    \caption{Cross entropy loss during the validation for UNet model with different parameters.}
    \label{fig:val_loss}
\end{figure}

Despite the fact that the largest model shows the lowest error value during the training process, the best model based on the metric values is UNet with started number of filters=16, the number of blocks=3, kernel size=5, with metrics score 300. Thus we can see that the graph on the validation sample does not correlate with the distance values, it can be concluded that the weighted cross-entropy is not quite the right choice of loss for the given task, it is likely that the replacement of this loss may bring a noticeable improvement in quality.

\begin{center}
\begin{table}
\centering
\makebox[0pt][c]{\parbox{0.9\textwidth}
{
\begin{minipage}[b]{1.0\linewidth}\centering
 \begin{tabular}{|| c || c | c | c | c ||}
 \hline
 UNet Params & F1 Score & TPR & std & Distance\\[0.5ex]
 \hline\hline
 F=8 KS=3 NB=3 & 0.533 & 0.369 & 204 & 316\\
 \hline
 F=8 KS=3 NB=4 & 0.534 & 0.37 & 207 & 318\\
 \hline
 F=8 KS=3 NB=5 & 0.527 & 0.361 & 205 & 319\\
 \hline
 F=8 KS=5 NB=3 & 0.448 & 0.291 & 261 & 394\\
 \hline
 F=8 KS=5 NB=4 & 0.517  & 0.357  & 203  & 328\\
 \hline
 F=8 KS=5 NB=5 & 0.499 & 0.337 & 222 & 348\\
 \hline
 F=16 KS=3 NB=3 & 0.55 & 0.383 & \textbf{188} & 300.8\\
 \hline
 F=16 KS=3 NB=4 & 0.541 & 0.378 & 196 & 308\\
 \hline
 F=16 KS=3 NB=5 & \textbf{0.555} & \textbf{0.39} & 191 & \textbf{300.6}\\
 \hline
 F=16 KS=5 NB=3 & 0.528 & 0.364 & 202 & 317\\
 \hline
 F=16 KS=5 NB=4 & 0.364  & 0.37  & 198 & 310\\
 \hline
 F=16 KS=5 NB=5 & 0.523 & 0.372 & 203 & 317\\
 \hline
 \hline
\end{tabular}
\end{minipage}\hfill
}}\vspace*{2mm}
\caption{The result of UNet model training with different parameters. Here F is a number of filters, KS - kernel size and NB is a number of blocks.}
\label{table:unet_params}
\end{table}
\end{center}

% \begin{figure}[h!]
%     \centering
%     \includegraphics[width=\textwidth]{images/val_loss.png}
%     \caption{Validation loss during during the training process.}
%     \label{fig:val_loss}
% \end{figure}

\subsection{FoCNN}

We tested several different architectures of FoCNN as well. Number of layers turned out to be crucial for performance of the neural network. The architecture presented in the Table \ref{focnn1} has a metrics score of 360 that is close to a simple CNN with 3 layers. Its value does not improve during training computed over the validation dataset.

BatchNormalization added to a final architecture plummets the metrics score to 340.

\begin{table}[!htb]
    
    \begin{subtable}
      
      \centering
 \begin{tabular}{|| c | c | c | c | c ||}
 \hline
 Layer  & KernelSize & Stride & Padding & Activ \\ [0.5ex]
 \hline\hline
 Conv. & 5x5 & 1 & 2 & ReLu \\
 \hline
        \end{tabular}
        
    \end{subtable}%
    \bigskip
    \begin{subtable}
      \centering
        
 \begin{tabular}{|| c | c | c | c | c ||}
 \hline
 Layer  & KernelSize & Stride & Padding & Activ \\ [0.3ex]
 \hline\hline
 Conv. & 5x5 & 1 & 2 & ReLu \\

 \hline
 Conv. & 3x3 & 1 & 2 & ReLu \\
 \hline
 Fc. & - & - & - & Sigmoid \\
 \hline
        \end{tabular}
        
    \end{subtable} 
    \caption{FoCNN$_{0}$ feature extractors.}
    \label{focnn1}
\end{table}
\if 0
\newpage
\subsection{Confusion matrices}

Here we present confusion table for test and extended data set. It is the same data set as previously, all sets were generated with the same rules. The source is found, as previously, if within 1.6 pixels from it there is a real source. This radius corresponds to a standard Fermi Telescope error. 

\begin{table}[H]
    
    \begin{subtable}
      
      \centering
 \begin{tabular}{|| c || c | c ||}
 \hline
 & Predicted  & Not predicted \\ [0.5ex]
 \hline\hline
Sources & 1770 & 1894 \\
\hline
No source & 115 & 1.6e+7 \\
 \hline
        \end{tabular}
        
    \end{subtable}%
    \bigskip
    \begin{subtable}
      \centering
        
 \begin{tabular}{|| c || c | c ||}
 \hline
 & Predicted  & Not predicted \\ [0.5ex]
 \hline\hline
Sources & 4070 & 4184 \\
\hline
No source & 233 & 3.6e+7 \\
 \hline
        \end{tabular}
        
    \end{subtable} 
    \caption{FoCNN$_{0}$ confusion table on test set and extended data set.}
    \label{focnn1}
\end{table}

\begin{table}[H]
    
    \begin{subtable}
      
      \centering
 \begin{tabular}{|| c || c | c ||}
 \hline
 & Predicted  & Not predicted \\ [0.5ex]
 \hline\hline
Sources & 1408 & 2256 \\
\hline
No source & 42 & 1.6e+7 \\
 \hline
        \end{tabular}
        
    \end{subtable}%
    \bigskip
    \begin{subtable}
      \centering
        
 \begin{tabular}{|| c || c | c ||}
 \hline
 & Predicted  & Not predicted \\ [0.5ex]
 \hline\hline
Sources & 3220 & 5034 \\
\hline
No source & 318 & 3.6e+7 \\
 \hline
        \end{tabular}
        
    \end{subtable} 
    \caption{UNet confusion table on test set and extended data set.}
    \label{focnn1}
\end{table}
\fi
